# Supplementary material for: Generalized Pose Space Embeddings for Training In-the-Wild using Anaylis-by-Synthesis
Source: arXiv:2411.08603 source file (2024-11-13)
Supplement: Supplementary file 1 [file body_supp.tex]

\section*{Appendix}
This supplementary material provides further evaluations and technical details. We provide additional comparisons on the Human3.6M~\cite{h36m:pami} dataset and further implementation details regarding model, training and hyperparameters.

\appendix
\section{Evaluation - Human3.6M}
Additionally to the results from the main paper, we provide a comparison of the median of the squared errors on the Human3.6M~\cite{h36m:pami} dataset, since the mean error (MSE) is sensitive to outliers and a few large errors can substantially influence the overall result. As in the main paper we show the results when ignoring flipped predictions in the metric as in \cite{Jakab:2020:CVPR} (\tabref{tab:Human3.6M:IgnoreFlipMedian}) as well as when considering flips (\tabref{tab:Human3.6M:WithFlipMedian}). Since the prior work of Jakab \etal~\cite{Jakab:2020:CVPR} does not provide the median, we cannot directly compare. 

From the metrics in \tabref{tab:Human3.6M:IgnoreFlipMedian} and \tabref{tab:Human3.6M:WithFlipMedian} we can observe a lower median error, comapred to the MSE, suggesting that there are some outliers present. While for the single-channel representation we observe a large difference, for our multi-channel skeleton image the difference is much smaller, showing that it is more robust (\ie more accurate for harder cases). Furthermore, for the refined model the difference is even smaller, indicating that the instance-specific refinement step significantly improves the accuracy on hard cases. Similar to the mean error in the main paper, from the differences between \tabref{tab:Human3.6M:IgnoreFlipMedian} and \tabref{tab:Human3.6M:WithFlipMedian} we observe that the multi-channel representation is less susceptible to flips compared to just a single channel.

\TableIgnoreFlipMedian
\TableConsiderFlipMedian

\section{Training Details}
During training we optimize several objectives, as described in the main paper. For the pretraining of the individual modules as well as the end-to-end training, we use different hyper parameters described next. 

For all steps (pretraining of individual modules and end-to-end training using real data) we use the Adam optimizer \cite{Adam}. The optimizer parameters are set to $\beta_1 = 0.9$ and $\beta_2 = 0.999$ during pretraining of the \textit{Skeleton Image Encoder}, the \textit{2D Pose Estimator} and the \textit{3D Uplift}. And for the pretraining of the \textit{Image Renderer} as well as the unsupervised end-to-end-training we use $\beta_1 = 0.5$ and $\beta_2 = 0.999$ and clip the norms of the gradients to 1.0 for stability. For all steps the learning rate is updated with an exponential decay with factor 0.95.

\subsection{Pretraining}
The learning rate and batch size are set to $2 \cdot 10^{-4}$ and 16 when pretraining the skeleton image encoder and the 2D pose estimator and $5 \cdot 10^{-4}$ and 100 respectively for the 3D uplifting. In all three cases we use L2 losses. For the 3D positions and orientations, the losses are balanced with the weights $w_{pos} = 10$ and $w_{orient} = 1$. Note that to ensure continuity in rotation space, we use the 6D representation from \cite{Zhou_2019_CVPR}. 

The image renderer is pretrained with a GAN setup similar to the unsupervised end-to-end training, with the render loss as described in the main paper. We chose a learning rate of $2 \cdot 10^{-4}$ with a batch size of 8. To balance the different loss terms we set the weights $w_{perc\_img} = 10$, $w_{disc\_img} = 1$ and $w_{disc\_img\_FM} = 10$.

\subsection{End-to-End Training}
The end-to-end training on unlabelled real data, together with some supervision from synthetic data requires more care for balancing all the different loss terms as they are at different scales. For the end-to-end training, we use a learning rate of $2 \cdot 10^{-5}$ with a batch size of 8. The weights for balancing the the loss terms of the synthetic supervision, as well as the unsupervised training on real data, are chosen as follows:
\paragraph{Synthetic supervision:}
\begin{align*}
    &w_{sk} = 100, \\
    &w_{pos\_2D} = 100, \\
    &w_{pos\_3D} = 100, \\
    &w_{orient\_3D} = 10.
\end{align*}
\paragraph{Unsupervised training on real data:}
\begin{align*}
    &w_{disc\_sk} = 10, \\
    &w_{rec\_sk} = 1000, \\
    &w_{rec\_sk\_proj} = 1000, \\
    &w_{perc\_img} = 10, \\
    &w_{disc\_img} = 1, \\
    &w_{disc\_img\_FM} = 10.
\end{align*}
Note that the Adam optimizer is invariant to the scale of the loss. Therefore, while the weights might seem large, it is only the relative scale that matters. Furthermore, the weights for the synthetic supervision might seem large, but their influence is still smaller due to differences in scale of the individual terms.

\section{Model Architecture}
The model architectures of the \emph{skeleton image encoder}, \emph{2D pose estimator} and \emph{image renderer} follow \cite{Jakab:2020:CVPR}, extended to support our multi-channel skeleton image. The architecture of the \emph{3D uplifting} module is based on \cite{Martinez17}. Each channel of the skeleton image is created similar as in \cite{Jakab:2020:CVPR} with the equation described in the main paper, which is fully differentiable and hence the gradients can flow through the analytic skeleton image module.

\section{Implementation Details}
The synthetic data was generated with the Unreal Engine \cite{unrealengine}. The model was implemented in PyTorch \cite{PyTorch} and trained on an RTX~2080~Ti.
